# Supplementary material for: Scenario Dreamer: Vectorized Latent Diffusion for Generating Driving Simulation Environments
Source: arXiv:2503.22496 source file (2025-03-28)
Supplement: Supplementary file 1 [file introduction.tex]

This supplementary document provides additional information to support the findings in the main manuscript. Specifically, we include additional quantitative and qualitative results, details of the proposed simulation framework, additional model details, and evaluation details. We encourage readers to visit our webpage for additional qualitative results and videos.
